# Supplementary material for: scX: A user-friendly tool for scRNA-seq exploration
Source: arXiv:2311.00012 source file (2024-03-07)

# scX: A user-friendly tool for scRNA-seq exploration

**Supplementary Material**

|                                                     | scX | ShinyCell | cellxgene | iSEE | UCSC Cell Browser | SCHNAPPs | SEQUIN | ShIVA | SingleCellAnalyzer | CellSnake | ASAP          | Loupe Browser |
|-----------------------------------------------------|-----|-----------|-----------|------|-------------------|----------|--------|-------|--------------------|-----------|---------------|---------------|
| SC analysis                                         | X   |           |           |      |                   | X        | X      | X     | X                  | X         | X             |               |
| SC analysis (interactive)                           |     |           |           |      |                   | X        | X      | X     | X                  |           | X             | X             |
| Web sharing                                         | X   | X         | X         | X    | X                 | X        | X      | X     | X                  |           | X             |               |
| Docker                                              | X   |           | X         | X    |                   |          |        | X     |                    | X         | X             |               |
| Cloud Support                                       | X   | X         | X         |      |                   | X        |        | X     |                    |           |               |               |
| SaaS                                                |     |           |           |      | X                 |          | X      |       | X                  |           | X             | X             |
| Dataset Summary                                     | X   |           |           |      |                   | X        | X      | X     |                    |           | X             | X             |
| QC plots                                            | X   |           |           |      |                   | X        | X      | X     | X                  |           |               |               |
| Explore covariates (categorical)                    | X   | X         | X         |      |                   | X        | X      | X     |                    |           |               |               |
| Explore covariates (continuous)                     | X   | X         | X         | X    |                   | X        | X      |       |                    |           |               |               |
| Multiple embeddings                                 | X   | X         | X         | X    | X                 | X        | X      | X     | X                  |           | X             | X             |
| 3D plots                                            | X   |           |           |      |                   | X        |        |       |                    |           | X             | X             |
| Interactive plots                                   | X   |           | X         | X    | X                 | X        |        | X     | X                  |           | X             | X             |
| Side-by-side embeddings                             |     | X         |           | X    | X                 |          |        |       | X                  |           |               |               |
| Differential Expression                             | X   |           | X         |      |                   | X        | X      | X     | X                  |           | X             | X             |
| on-the-fly cell-selection for marker identification | X   |           | X         | X    |                   | X        | X      |       |                    |           | X             | X             |
| Gene Co-expression                                  | X   | X         | X         |      |                   | X        |        |       |                    |           | X             | X             |
| Input of ad-hoc gene list                           | X   |           |           |      |                   |          |        |       |                    |           |               | X             |
| Multiple genes bubbleplots / heatmaps               | X   | X         |           | X    | X                 | X        | X      |       | X                  |           |               | X             |
| Order heatmap by covariate (continuous)             | X   |           |           | X    |                   |          |        |       |                    |           |               |               |
| Order heatmap by covariate (categorical)            | X   |           |           | X    |                   | X        | X      |       | X                  |           |               | X             |
| Zoom in/out                                         | X   |           | X         | X    | X                 | X        |        | X     |                    |           | X             | X             |
| Export images PDF/PNG                               | X   | X         |           |      | X                 | X        | X      | X     | X                  |           | X             | X             |
| SCE object                                          | X   | X         |           | X    |                   | X        |        |       |                    |           |               |               |
| Seurat object                                       | X   | X         |           |      | X                 |          |        | X     |                    |           |               | X             |
| txt/csv                                             | X   | X         |           |      | X                 | X        | X      |       |                    |           | X             |               |
| h5ad file                                           |     | X         | X         |      | X                 |          |        |       |                    |           |               |               |
| loom file                                           |     | X         |           |      | X                 |          |        |       |                    |           | X             |               |
| cellRanger                                          | X   |           |           |      |                   |          |        | X     |                    | X         |               |               |
| Platform                                            | R   | R         | Python    | R    | Python            | R        | R      | R     | Webpage            | R/Python  | R/Java/Python | App/R         |

Table ST1 Comparison between scRNAseq analysis tools based on functionalities (orange), implemented analyses and plot versatility (blue), and supported input file formats (green). Features were selected in the spirit of the comparison presented by Ouyang and collaborators [Ouyang2021]. ‘SC analysis’ refers to the capability of entering a raw object and performing a complete single-cell analysis (normalization, dimReduction, clustering, marker selection); ‘interactive’ refers to the capability of conducting the whole analysis within the app. ‘Web-sharing’ refers to the ability to host the data on a web page. ‘Docker’ indicates whether a Docker image is included with the tool. ‘Cloud support’ indicates whether instructions are available to deploy the application on a public cloud. ‘SaaS’ (Software as a Service) indicates whether the tool is hosted, allowing users to upload their data and interactively process it.

| N         | Size     | Preprocess |             |         | Markers tab | Heatmap w/o cell clustering |             | Heatmap w/ cell clustering |             |
|-----------|----------|------------|-------------|---------|-------------|-----------------------------|-------------|----------------------------|-------------|
|           |          | scX size   | Memory (GB) | Time    | Memory (GB) | Memory (GB)                 | Approx time | Memory (GB)                | Approx time |
| 5000      | 126.5 MB | 619.8 MB   | 2.76        | 0:03:45 | 0.49        | 0.47                        |             | 2.92                       |             |
|           |          |            | 3.00        | 0:04:07 | 0.49        | 0.46                        | 0:00:04     | 2.80                       | 0:00:23     |
|           |          |            | 2.77        | 0:04:02 | 0.48        | 0.46                        |             | 2.72                       |             |
| 10000     | 228 MB   | 894.2 MB   | 3.55        | 0:07:43 | 0.55        | 0.29                        |             | 3.08                       |             |
|           |          |            | 3.86        | 0:08:02 | 0.54        | 0.49                        | 0:00:06     | 3.59                       | 0:00:35     |
|           |          |            | 3.33        | 0:08:02 | 0.54        | 0.49                        |             | 3.59                       |             |
| 20000     | 431 MB   | 2.7 GB     | 4.86        | 0:17:43 | 0.79        | 0.68                        |             | 5.34                       |             |
|           |          |            | 4.86        | 0:17:45 | 0.86        | 0.68                        | 0:00:05     | 5.89                       | 0:01:15     |
|           |          |            | 5.34        | 0:17:46 | 0.86        | 0.68                        |             | 5.89                       |             |
| 40000     | 837.8 MB | 4 GB       | 6.34        | 0:36:44 | 1.17        | 0.8                         |             | 4.00                       |             |
|           |          |            | 6.34        | 0:38:50 | 1.19        | 0.9                         | 0:00:10     | 4.02                       | 0:03:06     |
|           |          |            | 6.26        | 0:38:56 | 1.19        | 0.8                         |             | 4.00                       |             |
| 80000     | 1.9 GB   | 8.1 GB     | 11.70       | 1:33:35 | 2.11        | 1.03                        |             | 12.09                      |             |
|           |          |            | 12.02       | 1:25:52 | 2.04        | 1.07                        | 0:00:16     | 12.05                      | 0:07:16     |
|           |          |            | 11.94       | 1:26:13 | 2.04        | 1.07                        |             | 10.52                      |             |
| 160796    | 3.3 GB   | 12.4 GB    | 23.58       | 2:41:58 | 3.96        | #N/A                        |             | #N/A                       | #N/A        |
|           |          |            | 23.58       | 2:40:17 | 5.06        | #N/A                        |             | #N/A                       | #N/A        |
|           |          |            | 23.59       | 2:44:54 | 5.06        | #N/A                        |             | #N/A                       | #N/A        |
| 80000(*)  | 1.9 GB   | 8.1 GB     |             |         | 6.67        | 6.68                        | 0:00:14     | 11.30                      | 0:03:30     |
| 160796(*) | 3.3 GB   | 12.4 GB    |             |         | 7.4         | 7.4                         | 0:00:13     | 10.68                      | 0:03:00     |

Table ST2 scX running times and peak memory consumption for sub-sampled datasets from single-cell RNA-seq data from Zeisel et al. (2018). Tests (by triplicates) were performed in an Intel(R) Xeon(R) Silver 4116 CPU @ 2.10GHz with 514G total RAM. Number of cells for each subset (N) are displayed in the first column. The in-memory size of the initial R object (Size) and the object created by the preprocessing function (scX size) are shown in the second and third columns. Peak memory usage in GB and running time for the preprocessing step are shown in the 4<sup>th</sup> and 5<sup>th</sup> columns. The last 5 columns report these quantities for 3 different tasks performed in the interactive Shiny platform (Markers tab does not include duration because it involves interactive use). Heatmaps for the two larger datasets could not be generated at single-cell levels. The 2 final rows correspond to a random subsampling of 50k cells for plots in the app (default in scX for large datasets).

Details:

Preprocessing: Data was preprocessed with 3 partitionVars arguments ("Age", "Class", "OriginalClusters") for DEGs and markers analysis, and 1 metadataVars ("MitoRiboRatio").

Tab Markers -> Cluster markers: 3D scatter plot colored by partition, marker list for 1 cluster, expression plots for 1 marker gene (3D scatter plot by expression, violin and spike plots)

Tab EDA -> Fields: Heatmap for all fields (nCounts, nFeatures, MitoRiboRatio) with Cluster Row, without Cluster Column, colored by category "OriginalClusters"

Tab EDA -> Fields: Heatmap for all fields (nCounts, nFeatures, MitoRiboRatio) with Cluster Row and Cluster Column, colored by category "OriginalClusters"

## References:

Zeisel A et al. (2018). Molecular architecture of the mouse nervous system. Cell 174(4), 999-1014.  
<https://doi.org/10.1016/j.cell.2018.08.041>

Risso D, Cole M (2023). scRNAseq: Collection of Public Single-Cell RNA-Seq Datasets.  
<https://doi.org/10.18129/B9.2023.01>

R package version 2.16.0, <https://bioconductor.org/packages/2.16/bioc/html/scRNAseq/>

## Preprocess function

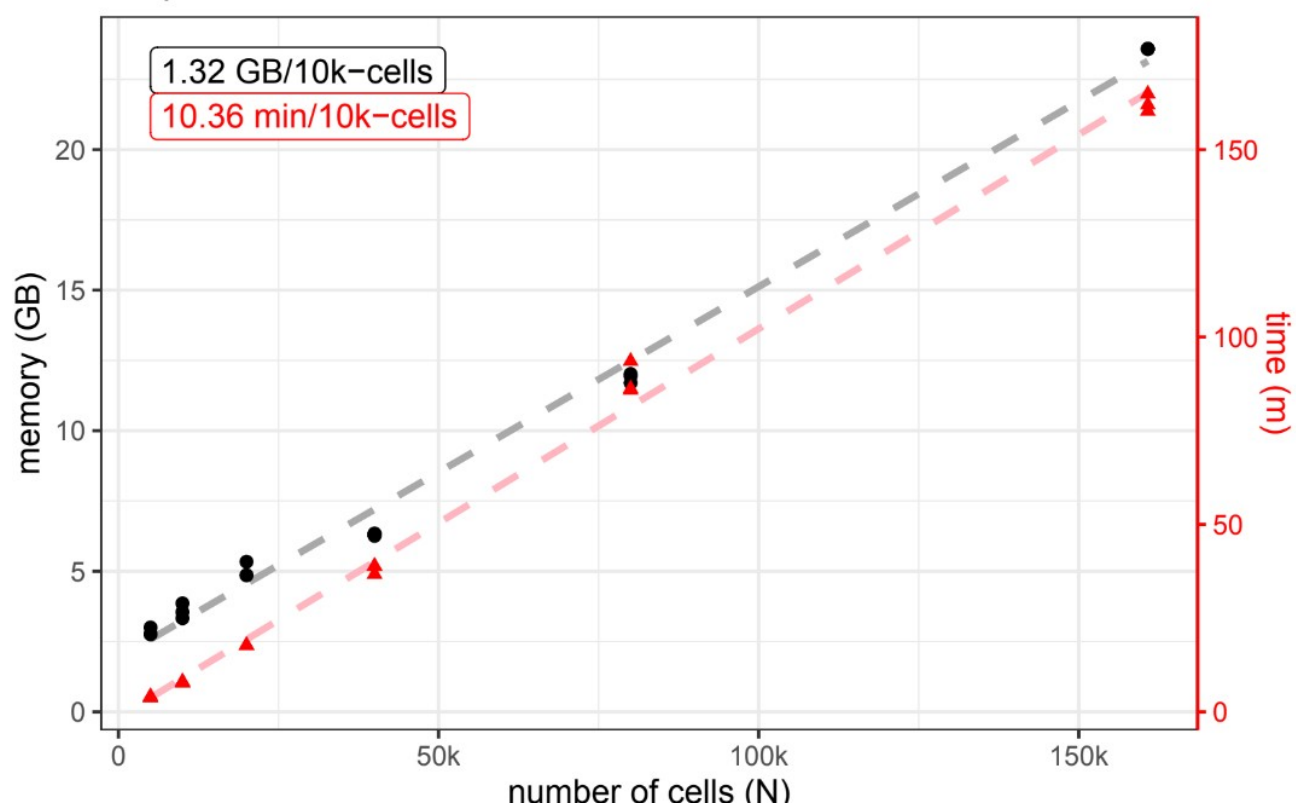

Supplement: Supplementary file 1 [file scX_supMat.pdf]
